# Supplementary material for: Cluster-Based Random Forest Visualization and Interpretation
Source: arXiv:2507.22665 ancillary file (2025-07-30)

---

# **SHORT SUMMARY OF RANDOM FORESTS**

# Decision tree

- Decision tree generated from data, most important nodes split on first.
- Path to leaf decides the class

| Age | Weight | Smoker | Risk |
|-----|--------|--------|------|
| 45  | 45     | Yes    | Yes  |
| 78  | 68     | Yes    | Yes  |
| 25  | 77     | Yes    | Yes  |
| 12  | 45     | No     | No   |
| 35  | 105    | No     | Yes  |
| 22  | 99     | Yes    | No   |
| 49  | 30     | No     | No   |

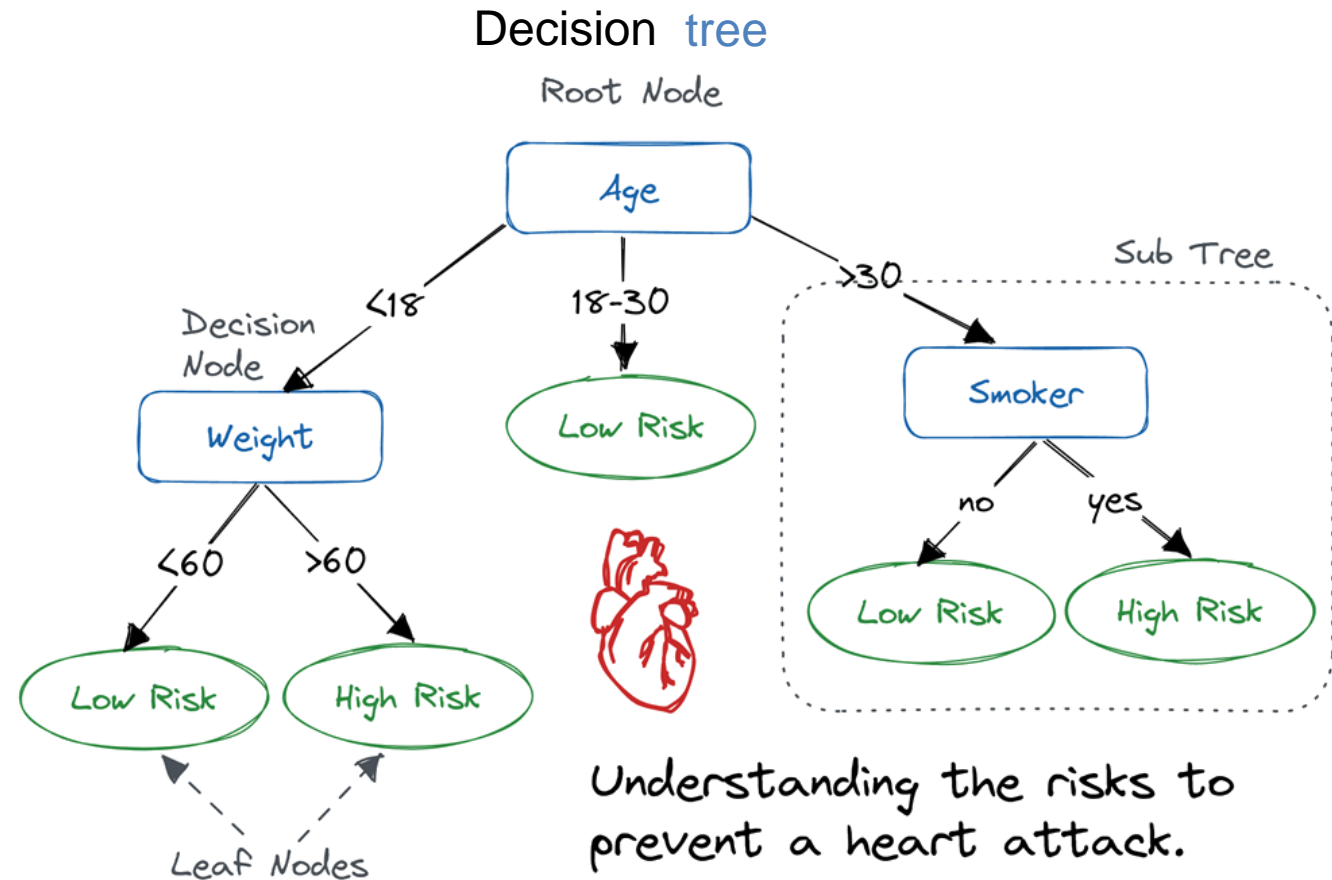

# Decision tree

- Danger of being overspecified
  - Learned exactly how to classify the input data
  - Doesn't generalize to new data

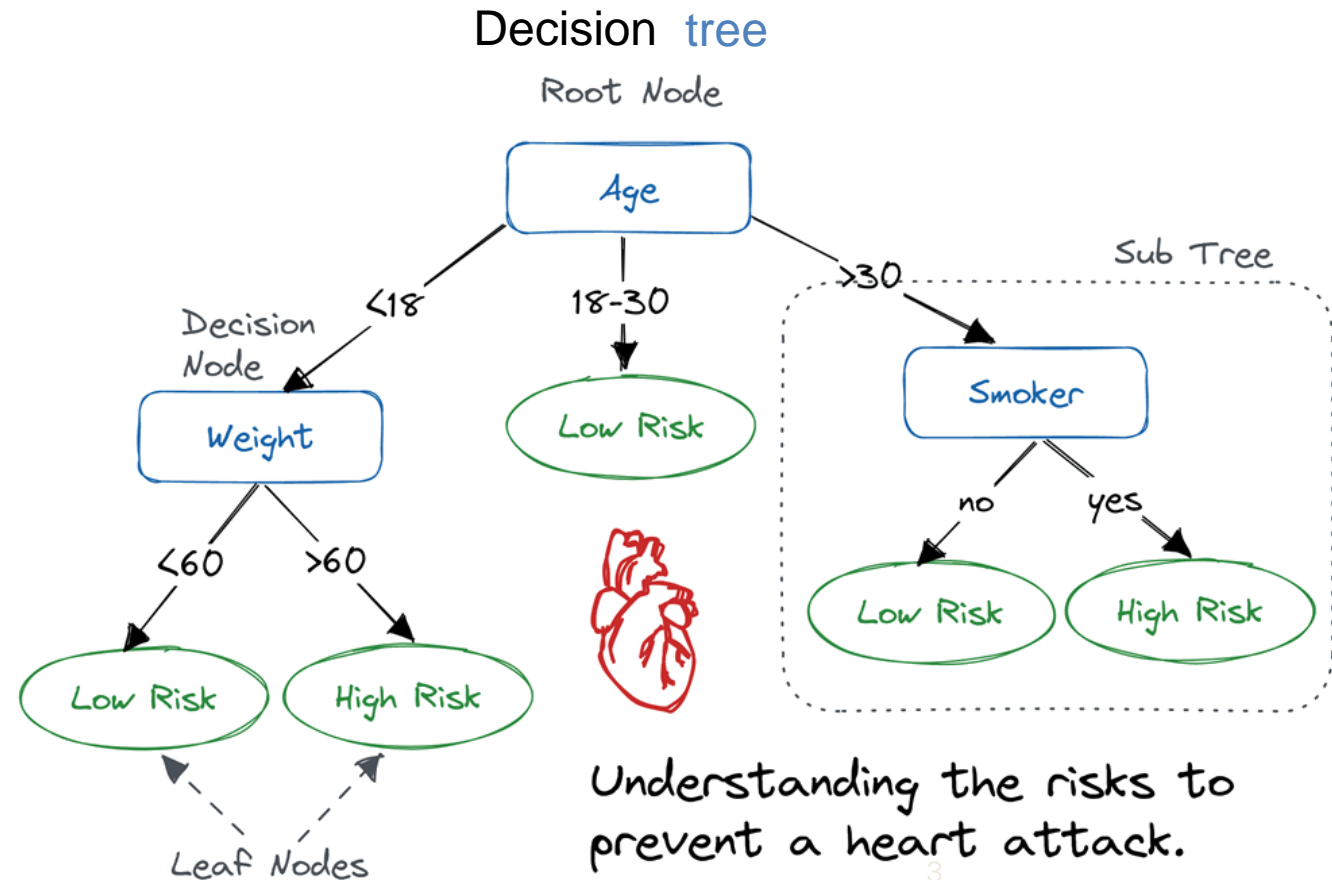

# Decision tree

- Danger of being overspecified
  - Learned exactly how to classify the input data
  - Doesn't generalize to new data
- Solution: Train many trees on part of input data
  - Use consensus to select label/class

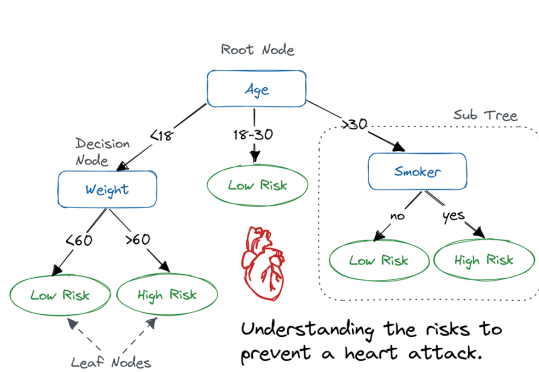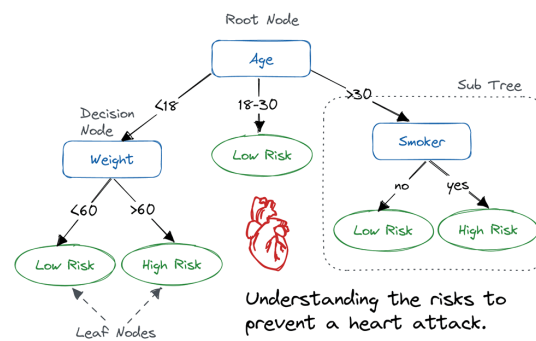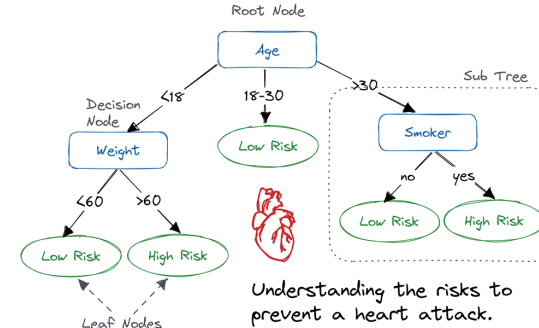

Random Forest

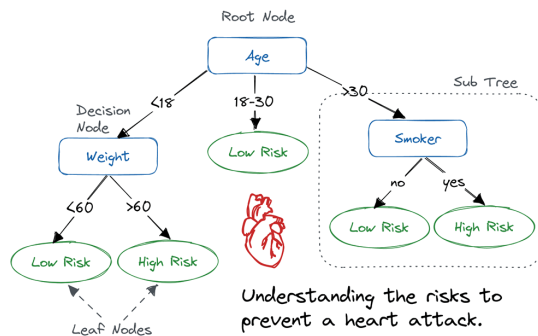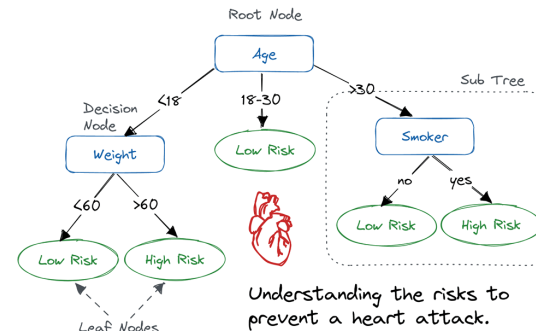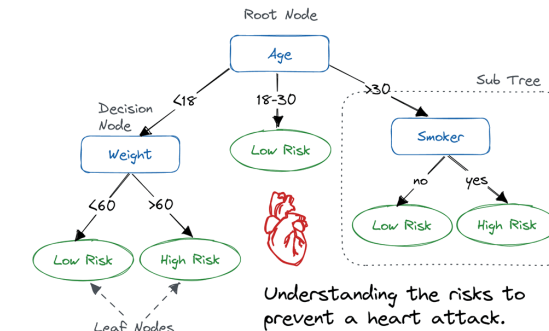

---

**NEW VISUALIZATION TO TEST**

---

# New Visualization

- Shows **clusters** of decisions trees in a random forest.
- Similar decision trees are put into the same cluster

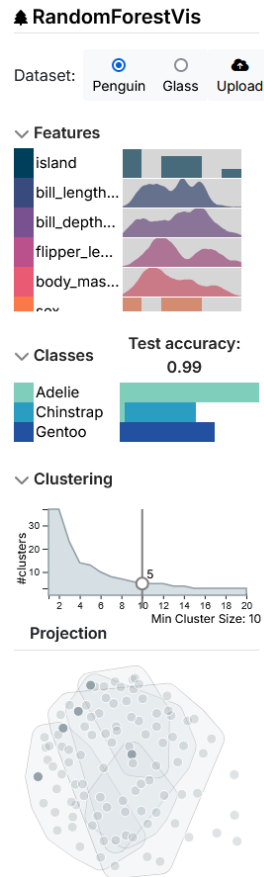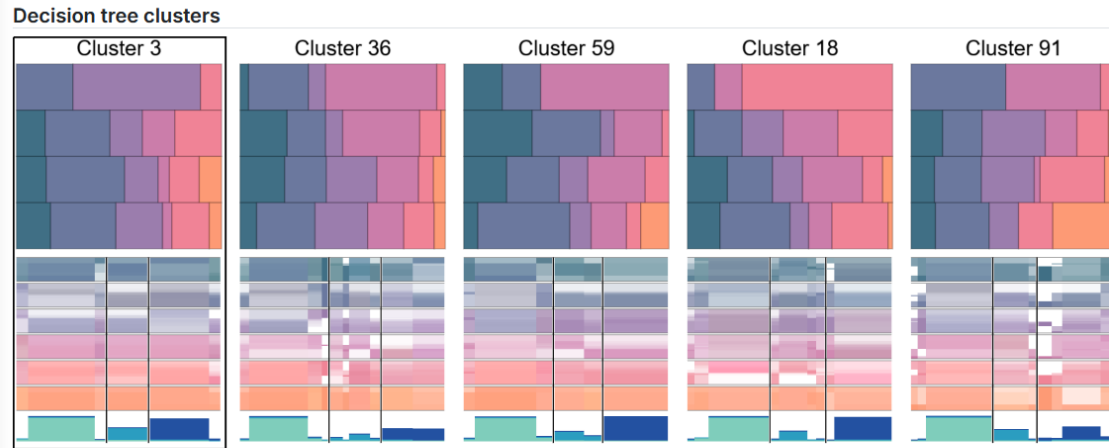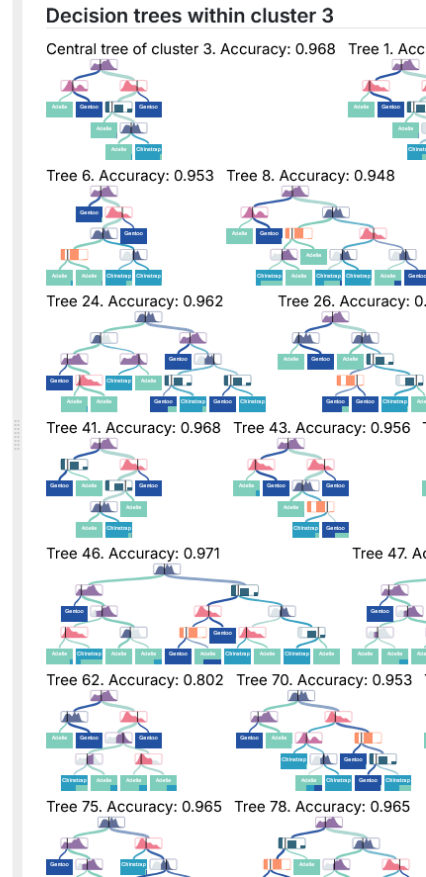

# New Visualization

- Shows **clusters** of decision trees in a random forest.
- Similar decision trees are put into the same cluster

## Global Information

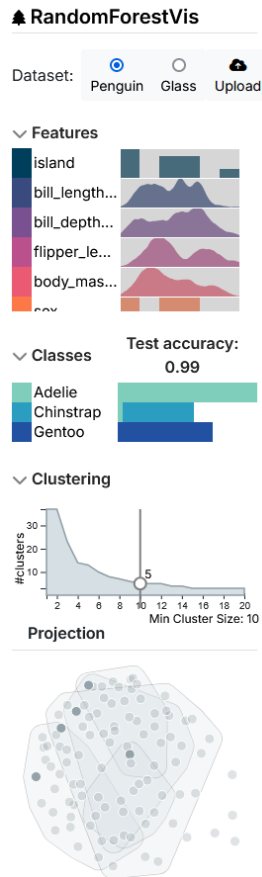

## Cluster Visualization

Decision tree clusters

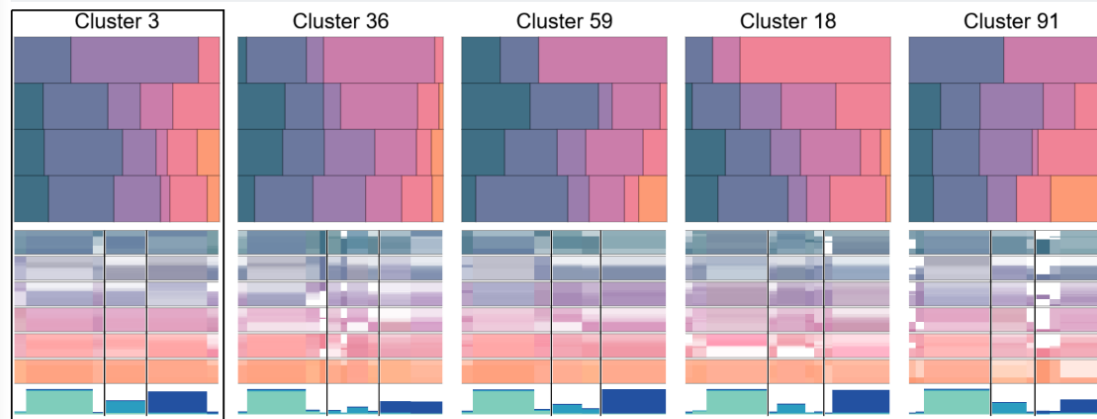

## Visualizing decision trees within a cluster

Decision trees within cluster 3

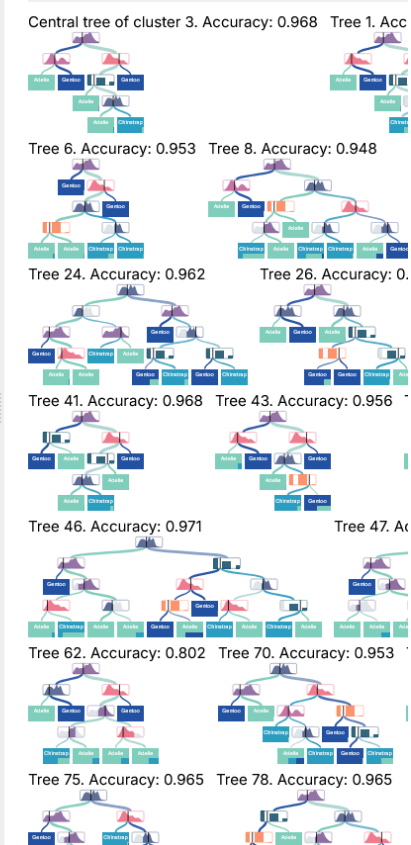

# New Visualization

Shows distribution of features

Shows distribution of Classes

## 🌲 RandomForestVis

Dataset:

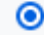

Penguin

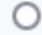

Glass

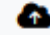

Upload

### Features

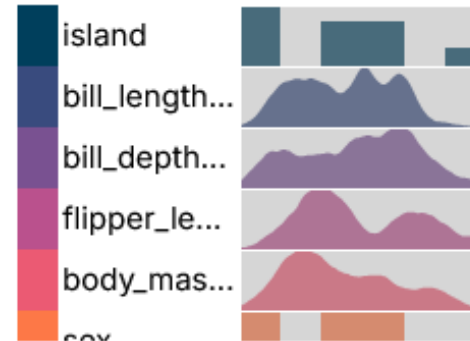

### Classes

Test accuracy:  
0.99

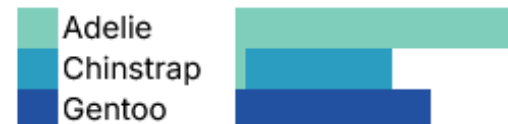



# New Visualization

Controls how large  
the clusters are

Gives an indication  
how similar trees  
within the clusters are

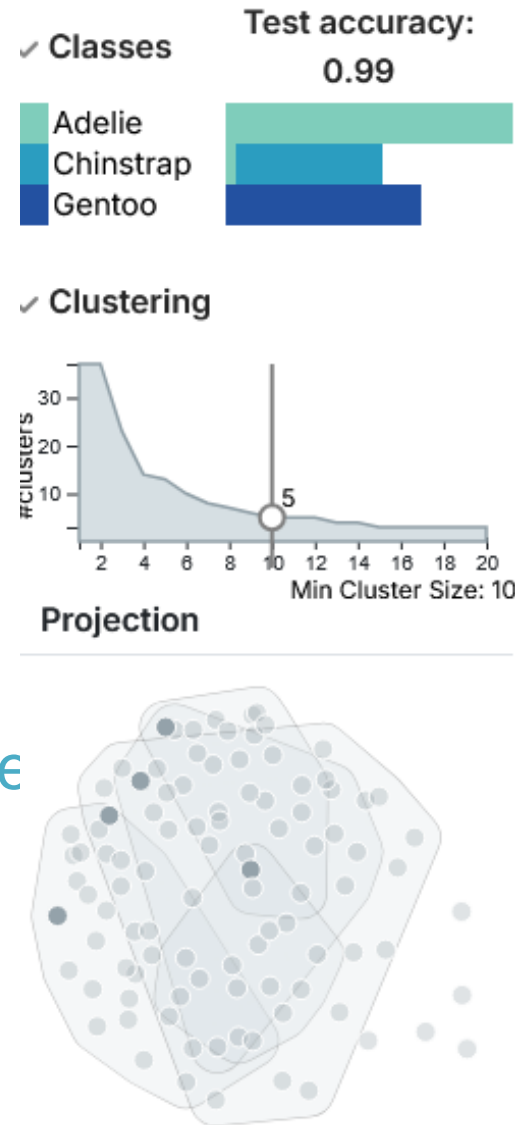

# New Visualization

Shows how often a feature is used within the cluster at a specific height in the tree.

Decision trees split on the most important feature per split.

-Most important features for a tree rise to the top.

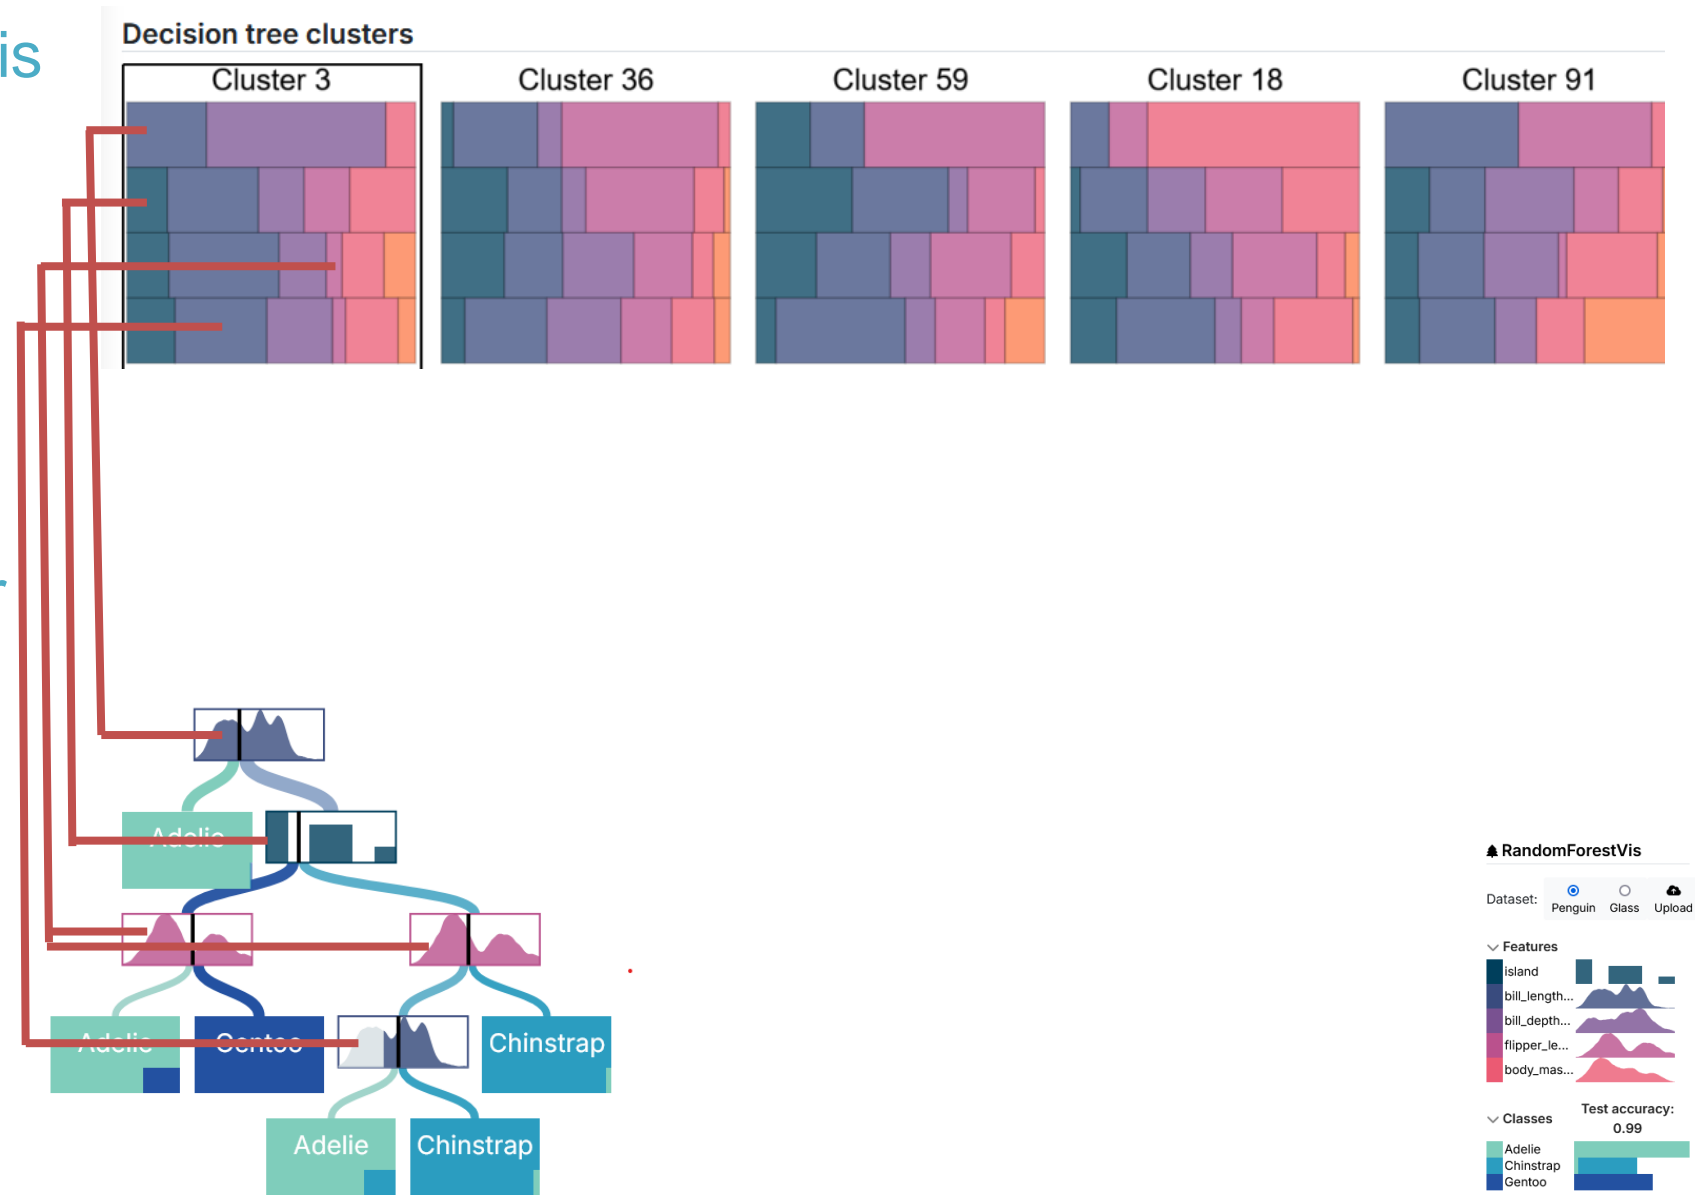

# New Visualization

Shows clustered classification rules (path to leaf node) used in this cluster.

Rules are grouped by similarity, frequency of usage and classification shown at the bottom.

Transparency is used when rules are similar but not exactly the same

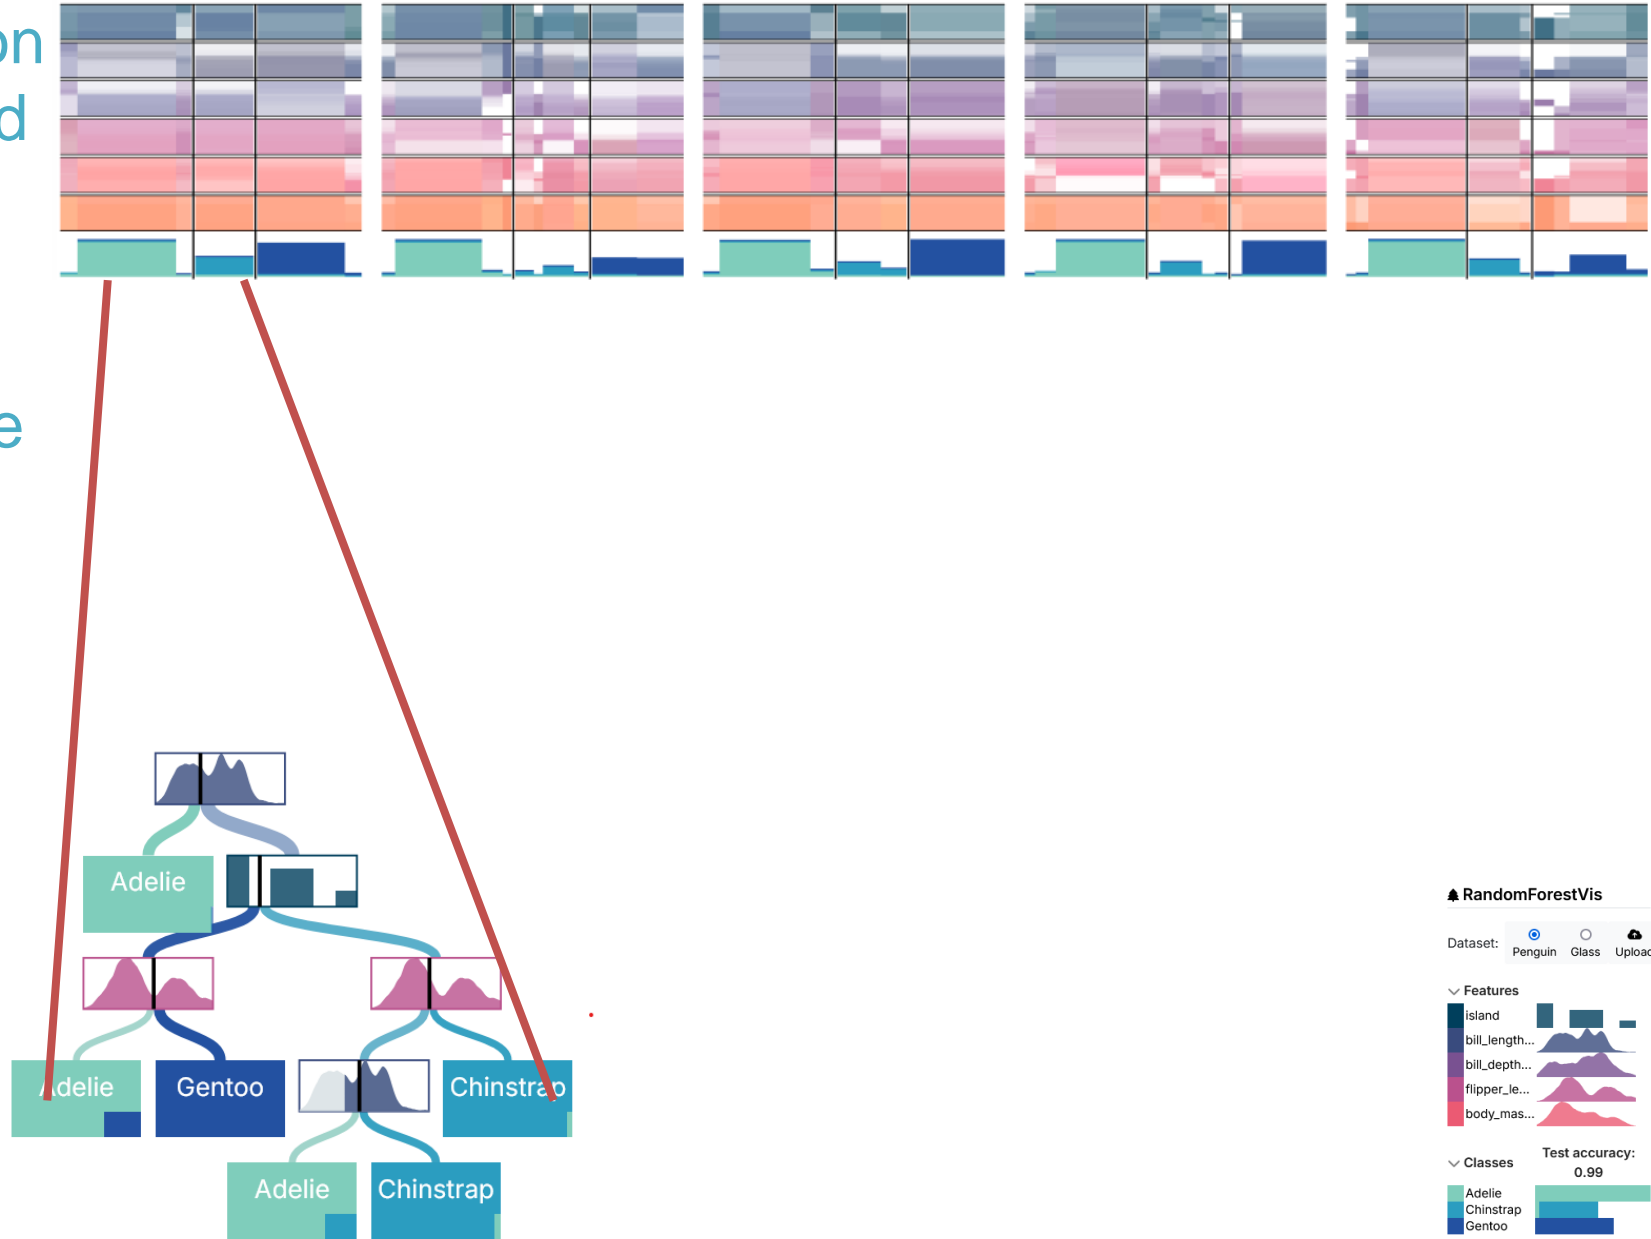

# New Visualization

Shows the decision trees within a cluster.

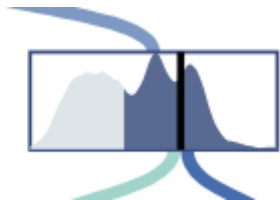

Nodes show the split point in black, and the feature distribution considered in this split in color.

Size of edges indicates how many paths go down each side of the splitpoint.

Classification matrix for a leaf node is shown underneath it

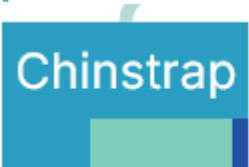

Centroid tree 59. Accuracy: 0.968 Tree Number 4. Accuracy: 0.965

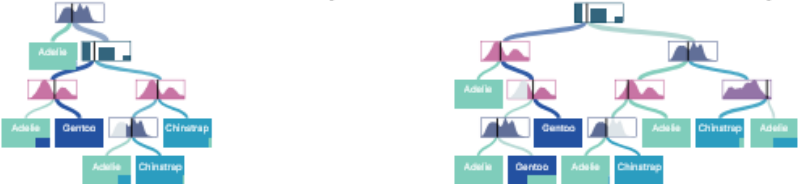

Tree Number 17. Accuracy: 0.936 Tree Number 20. Accuracy: 0.980

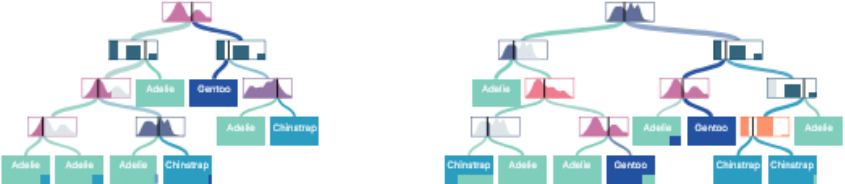

Tree Number 29. Accuracy: 0.837 Tree Number 31. Accuracy: 0.962

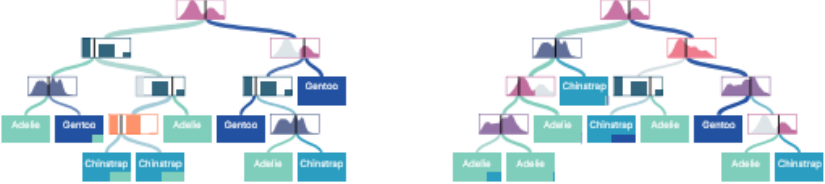

Tree Number 35. Accuracy: 0.971 Tree Number 60. Accuracy: 0.974

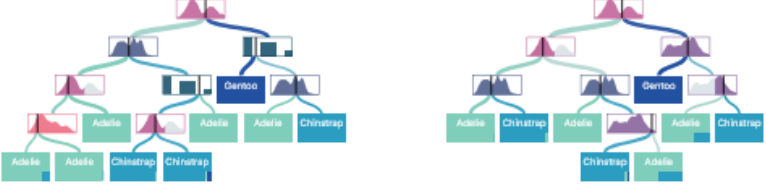

Tree Number 64. Accuracy: 0.971 Tree Number 68. Accuracy: 0.977

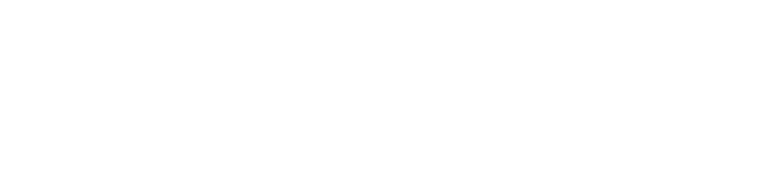

## RandomForestVis

Dataset: ☒ Penguin ☐ Glass

### Features

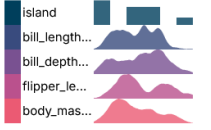

### Classes

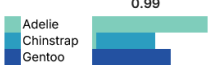

Test accuracy: 0.99

---

Held the link to the system.  
Removed for anonmization  
**SYSTEM DEMONSTRATION**

## Questions to answer

---

The following pages are NOT shown to the participant, and only there to help structure the interview.

# Questions to answer

- What are the most important features in the model?
  - Correct answer (in order of rough importance): Al (Aluminium), Mg (Magnesium), Ba (Barium)

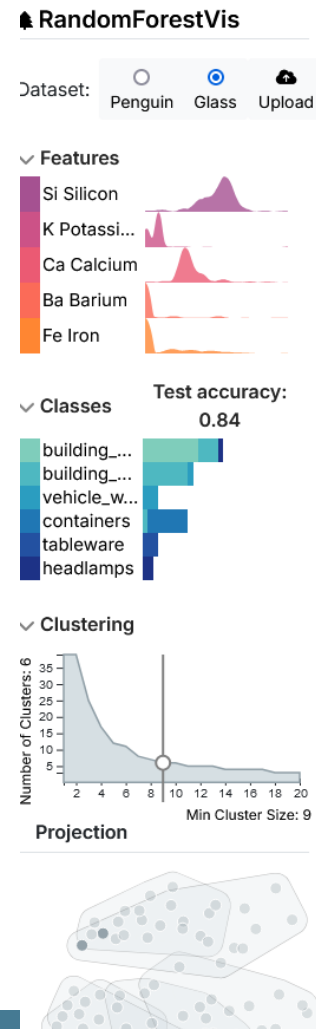

Decision tree clusters

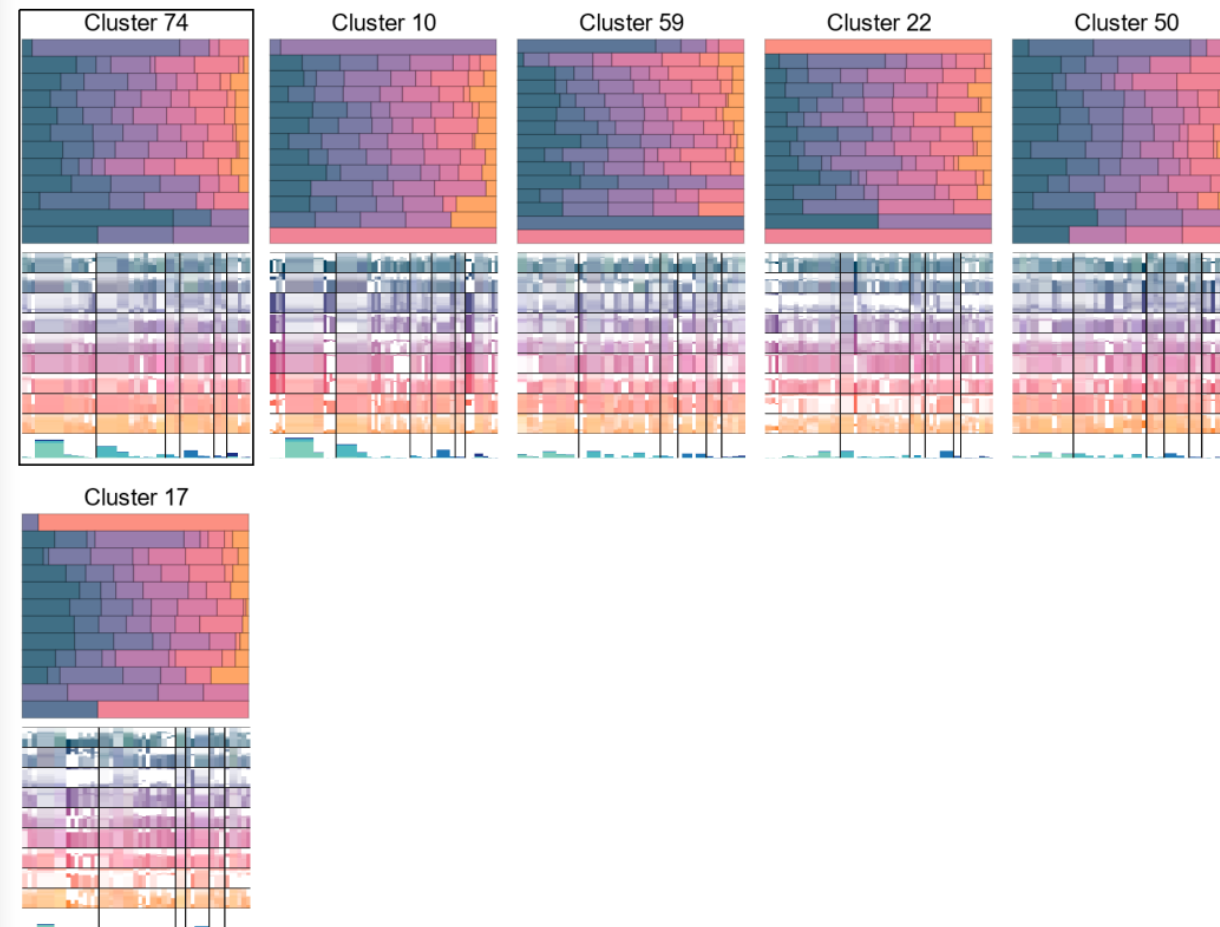

Decision trees within cluster

Centroid tree 74. Accuracy: 0.822

Tree Number 1. Accuracy: 0.855

Tree Number 5. Accuracy: 0.813

Tree Number 8. Accuracy: 0.850

Tree Number 9. Accuracy: 0.785

Tree Number 12. Accuracy: 0.808

Tree Number 21. Accuracy: 0.780

Tree Number 26. Accuracy: 0.794

Tree Number 30. Accuracy: 0.864

Tree Number 43. Accuracy: 0.813

Tree Number 48. Accuracy: 0.799

# Questions to answer

- How well is the model performing
  - 84% accuracy. Most misclassifications between two type of building windows.

RandomForestVis

Dataset: ☐ Penguin ☒ Glass ☐ Upload

Features

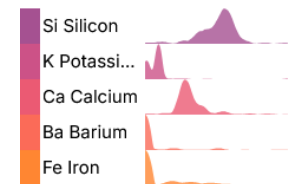

Classes

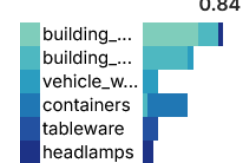

Test accuracy:  
0.84

Clustering

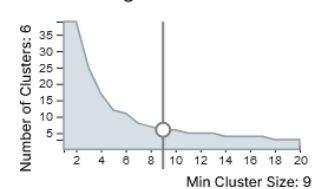

Projection

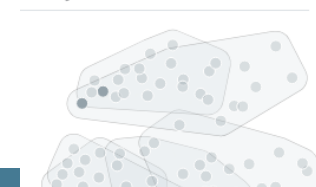

Decision tree clusters

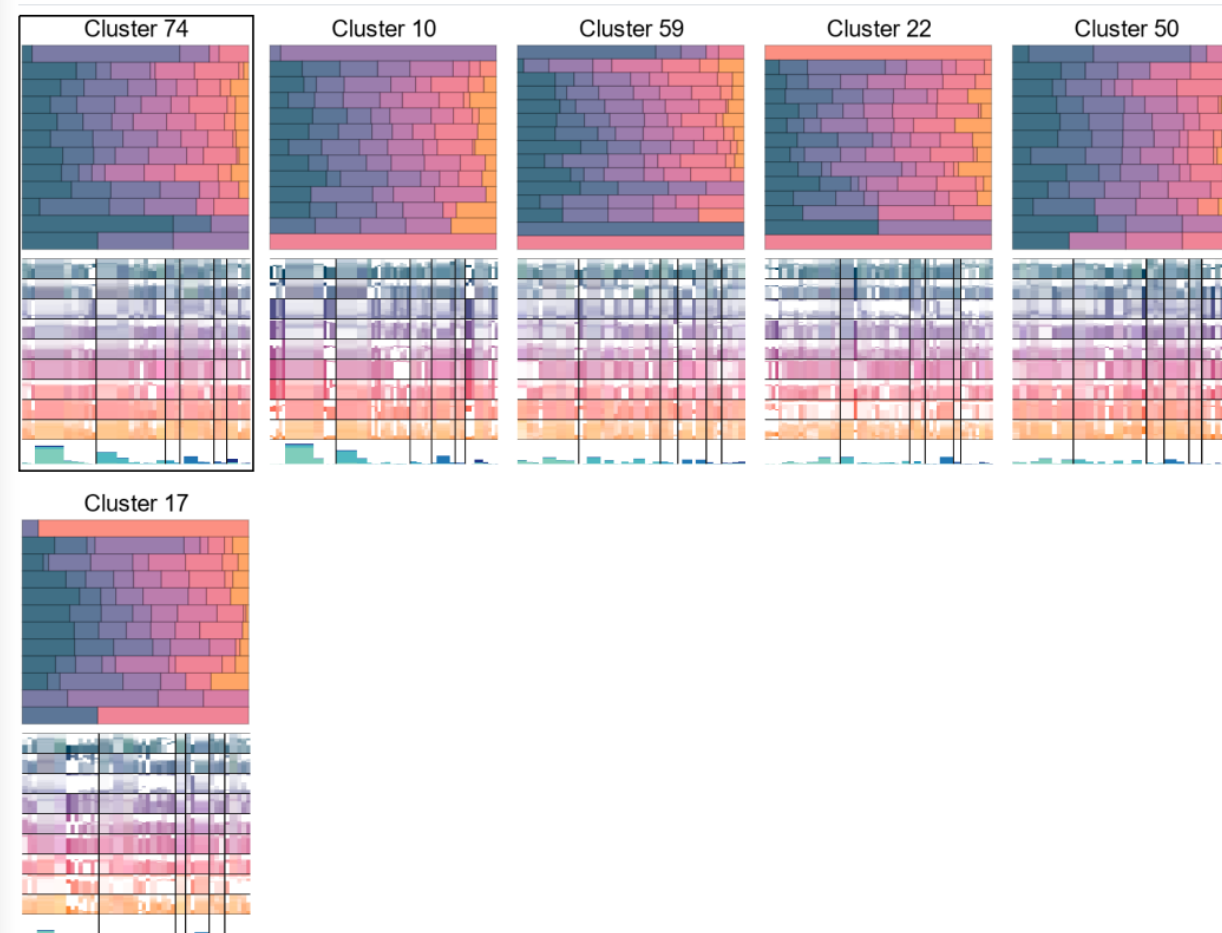

Decision trees within cluster

Centroid tree 74. Accuracy: 0.822

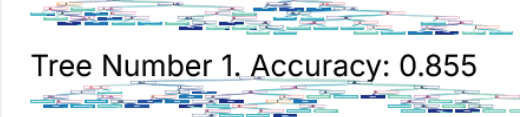

Tree Number 1. Accuracy: 0.855

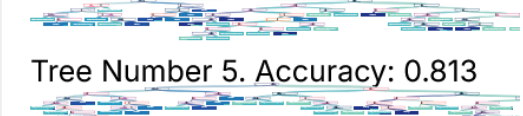

Tree Number 5. Accuracy: 0.813

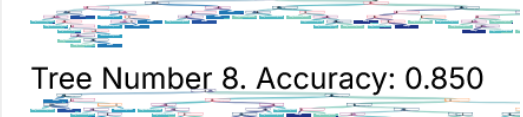

Tree Number 8. Accuracy: 0.850

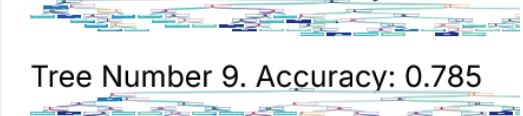

Tree Number 9. Accuracy: 0.785

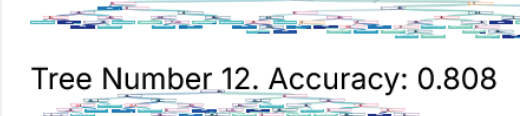

Tree Number 12. Accuracy: 0.808

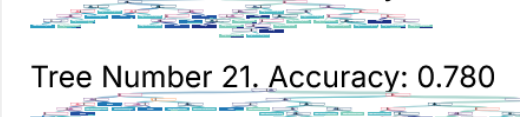

Tree Number 21. Accuracy: 0.780

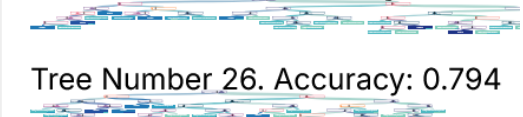

Tree Number 26. Accuracy: 0.794

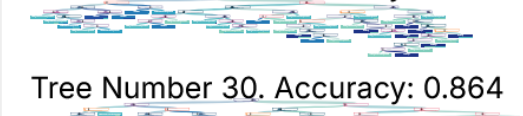

Tree Number 30. Accuracy: 0.864

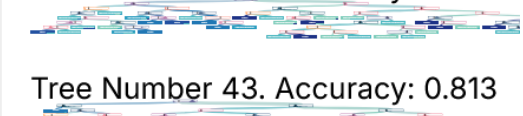

Tree Number 43. Accuracy: 0.813

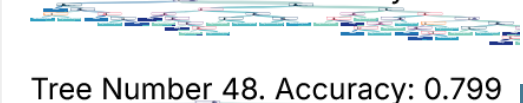

Tree Number 48. Accuracy: 0.799



# Questions to answer

- Which class is misclassified the most
  - Building\_windows\_Float\_processed  
(Misclassified into building\_windows\_non\_float\_processed)

RandomForestVis

Dataset: ☐ Penguin ☒ Glass ☐ Upload

Features

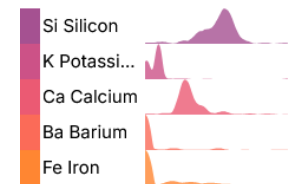

Classes

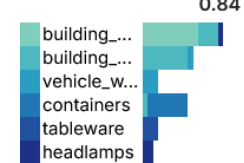

Test accuracy: 0.84

Clustering

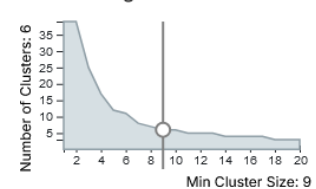

Projection

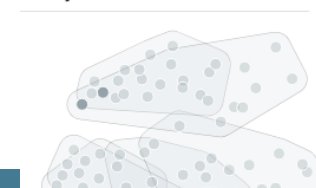

Decision tree clusters

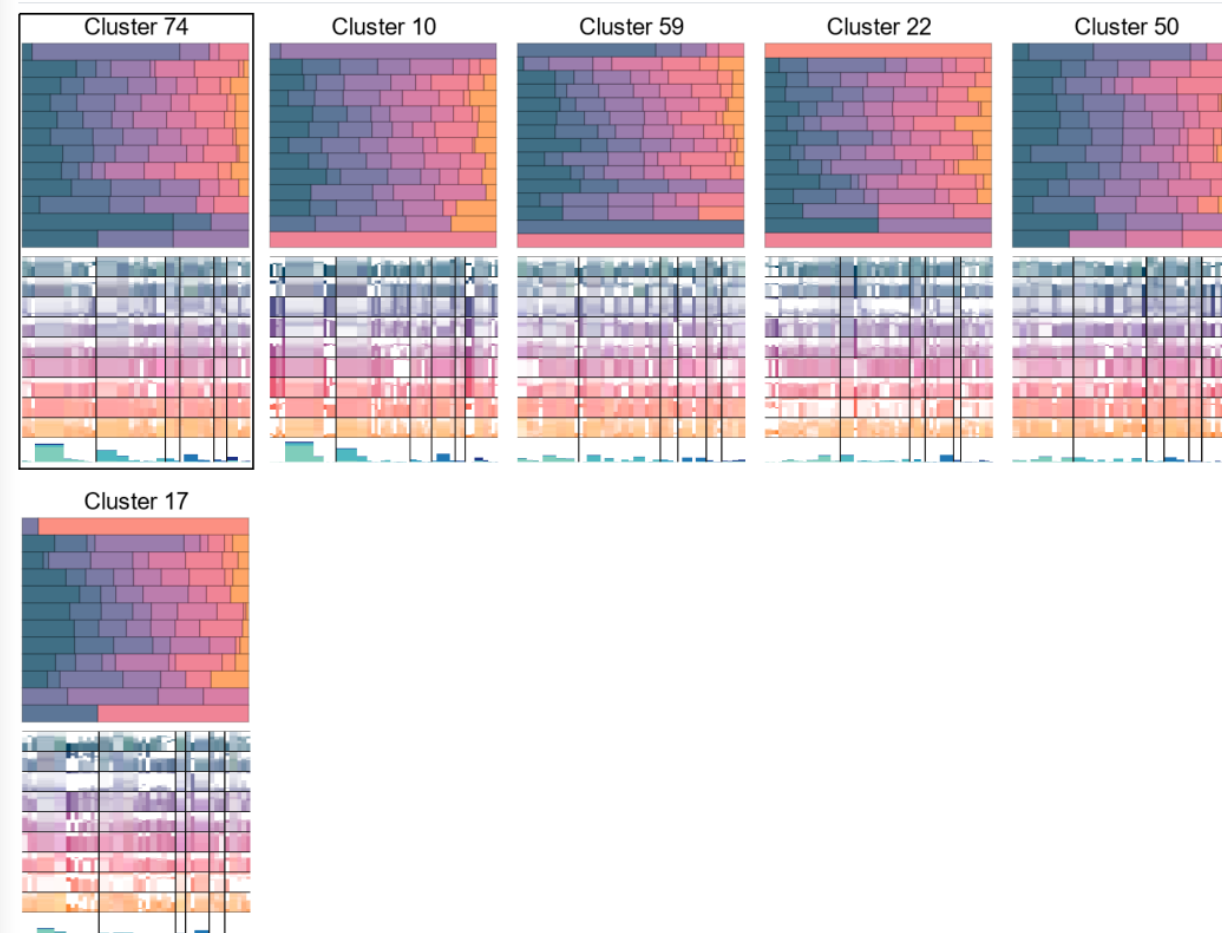

Decision trees within cluster

Centroid tree 74. Accuracy: 0.822

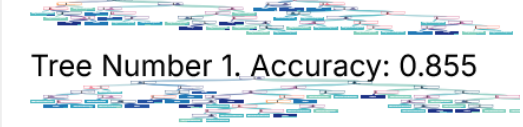

Tree Number 1. Accuracy: 0.855

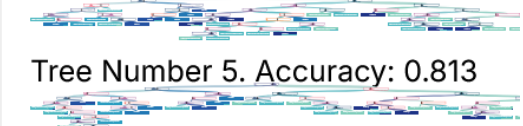

Tree Number 5. Accuracy: 0.813

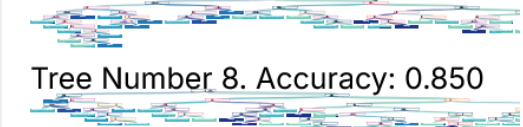

Tree Number 8. Accuracy: 0.850

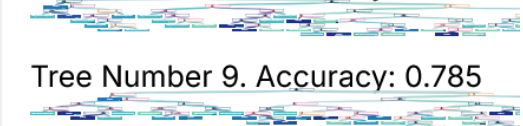

Tree Number 9. Accuracy: 0.785

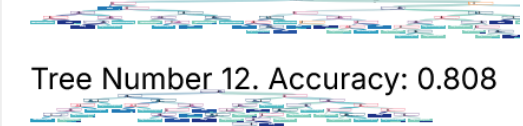

Tree Number 12. Accuracy: 0.808

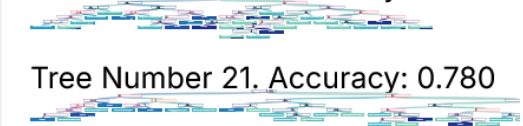

Tree Number 21. Accuracy: 0.780

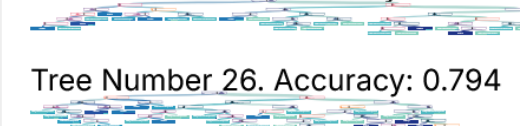

Tree Number 26. Accuracy: 0.794

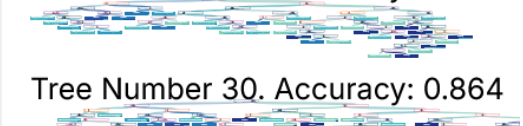

Tree Number 30. Accuracy: 0.864

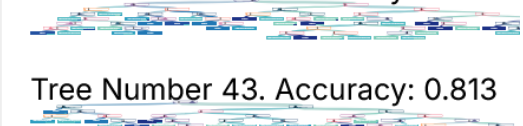

Tree Number 43. Accuracy: 0.813

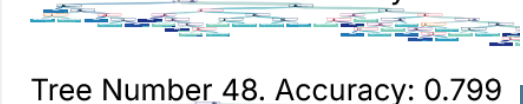

Tree Number 48. Accuracy: 0.799

# Questions to answer

- How does the model decide that an instance belongs to class “headlamps”?
- Minimum calcium level, high magnesium content, Minimum sodium level. At least medium silicon

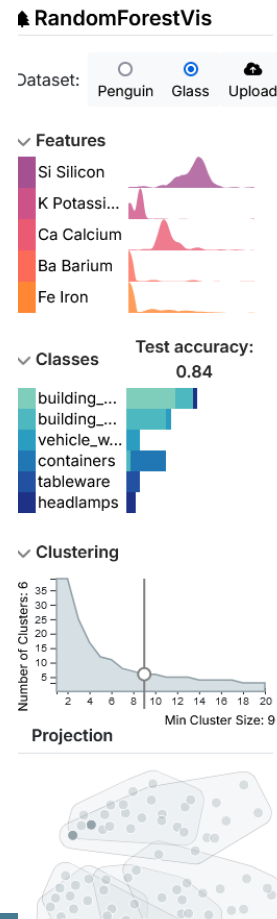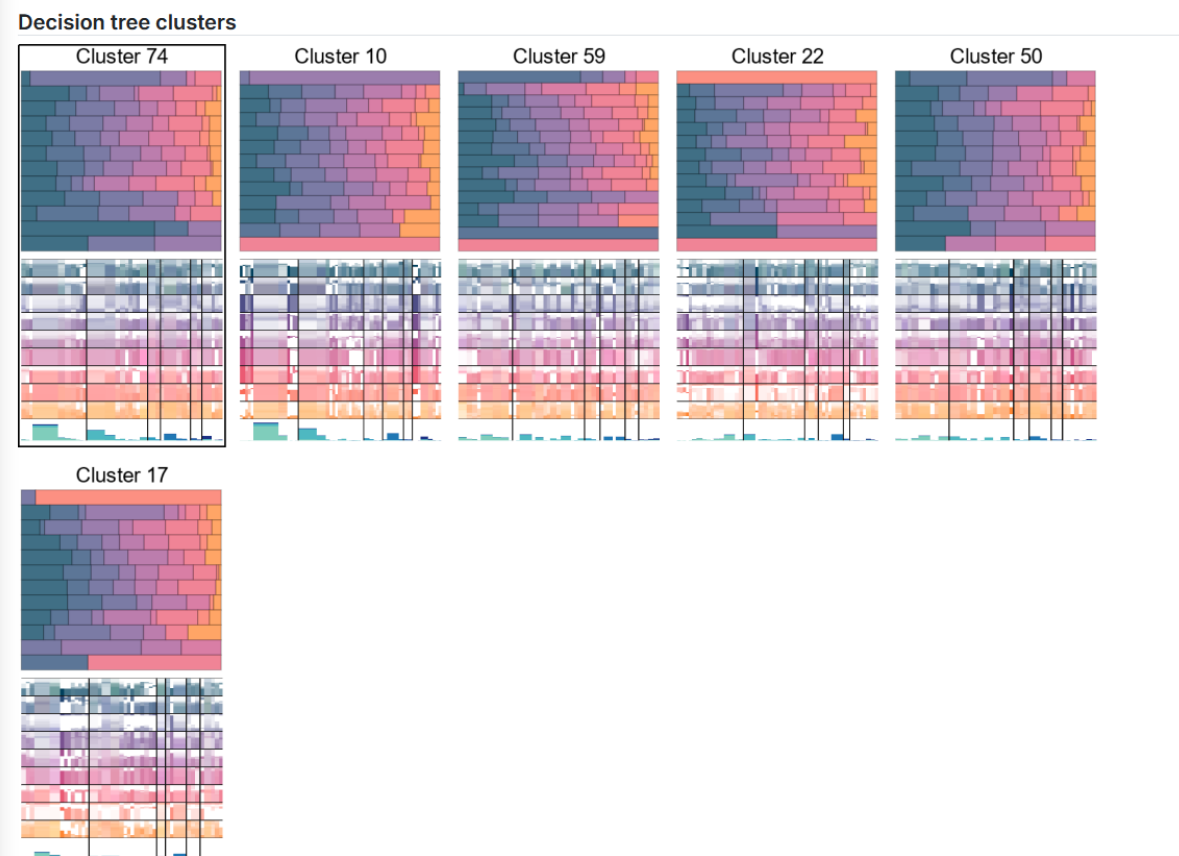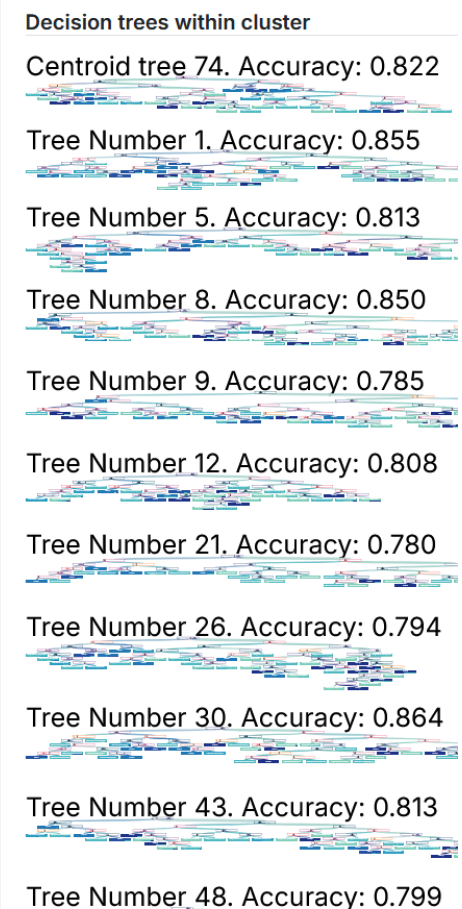

# Questions to answer

- What are the factors resulting in misclassification of class “Building”
  - Very important for this one: Why?

## RandomForestVis

Dataset: ☐ Penguin ☒ Glass ☐ Upload

### Features

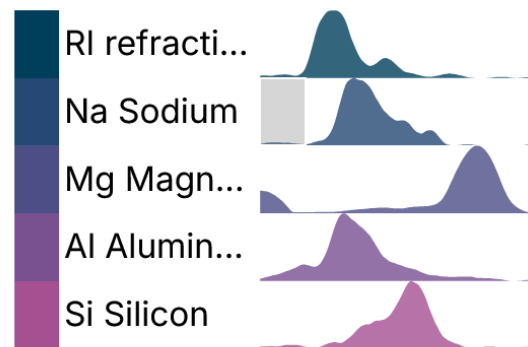

### Classes

building

Test accuracy:  
0.84

## Decision tree clusters

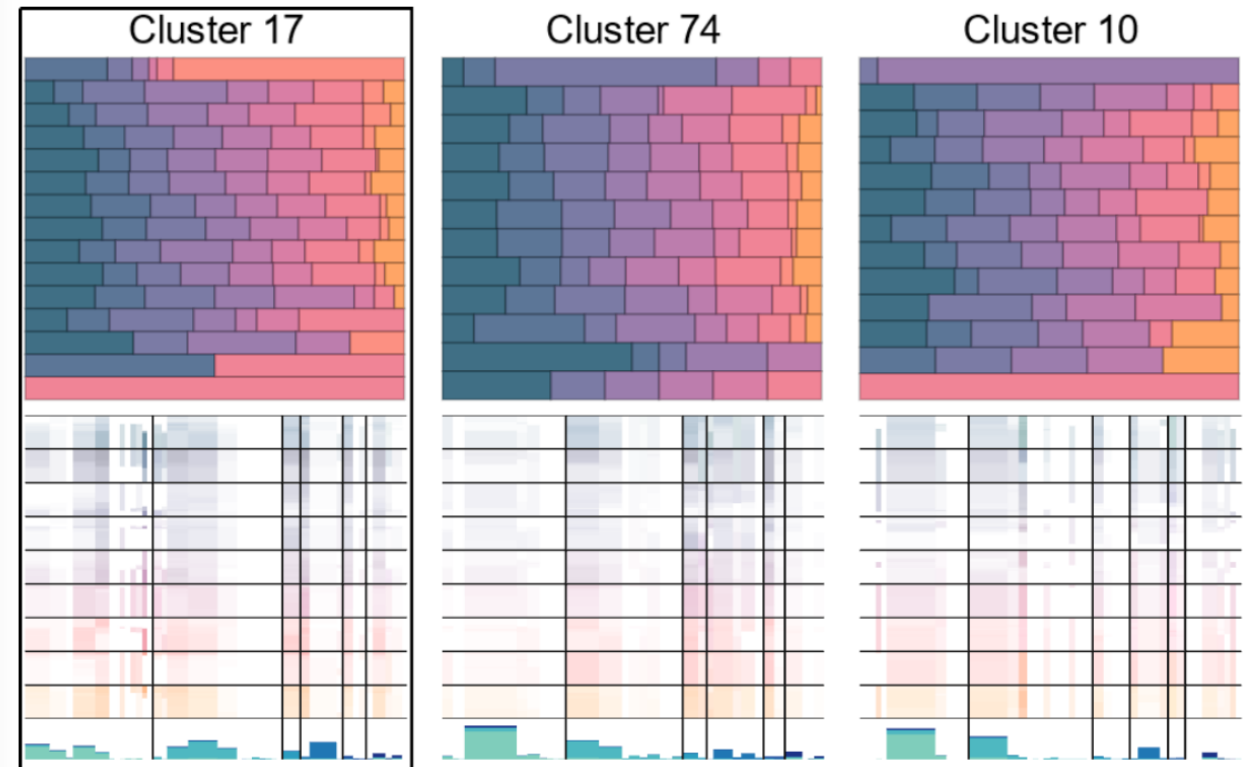

# Questions to answer

- How representative are the clusters shown of the underlying decision forest?

Different based on features plots

Projection

Min Cluster Size: 20

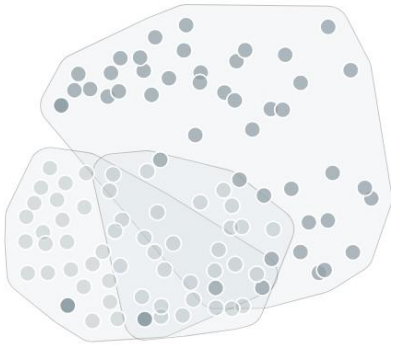

Projection

Min Cluster Size: 20

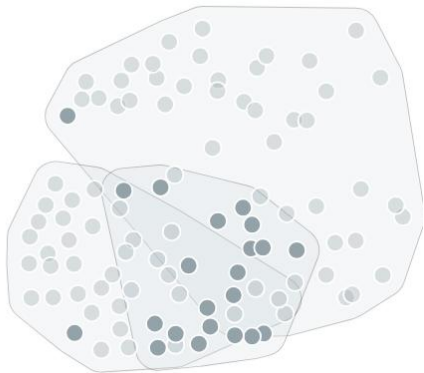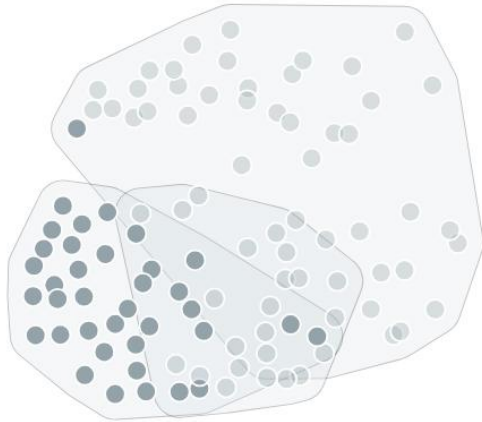

Cluster 17

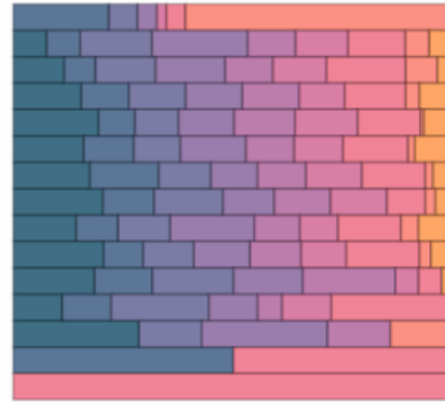

Cluster 74

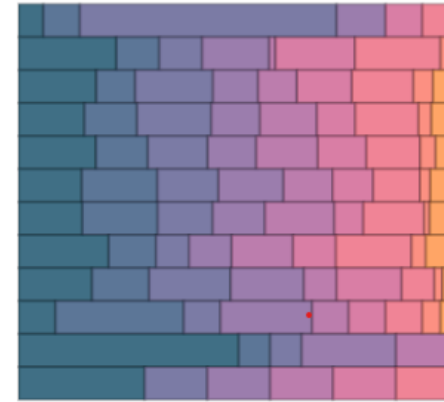

Cluster 10

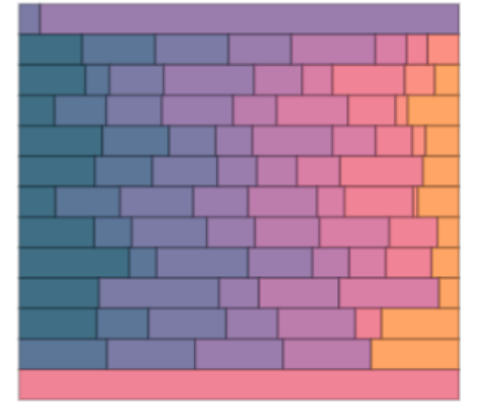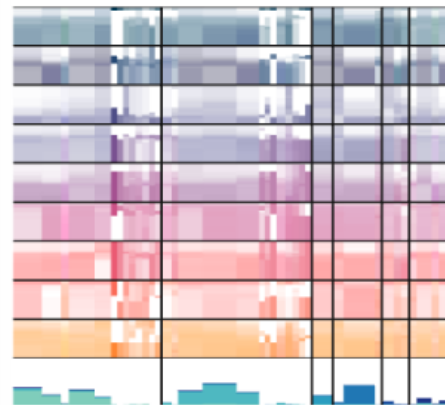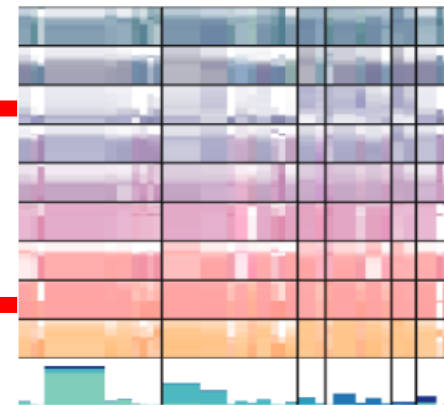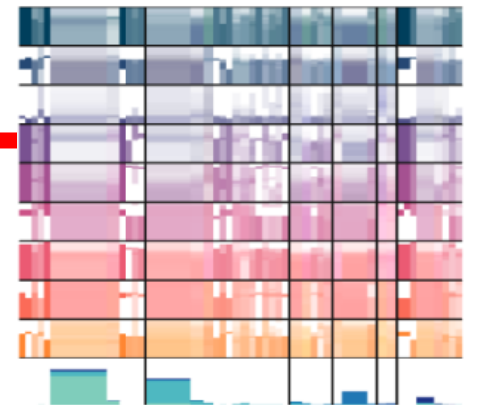

Supplement: Supplementary file 1 [file IntroductionToStudy+Questions.pdf]
