# Supplementary material for: Cluster-Based Random Forest Visualization and Interpretation
Source: arXiv:2507.22665 ancillary file (2025-07-30)
Supplement: Supplementary file 2 [file SurveyQuestions.pdf]

# Usability survey

Usability survey

\* Indicates required question

1. \*

Mark only one oval per row.

|                                                                                                   | 1<br>Strongly<br>Disagree | 2                     | 3                     | 4                     | 5<br>Strongly<br>Agree |
|---------------------------------------------------------------------------------------------------|---------------------------|-----------------------|-----------------------|-----------------------|------------------------|
| <b>I think that I would like to use this system frequently.</b>                                   | <input type="radio"/>     | <input type="radio"/> | <input type="radio"/> | <input type="radio"/> | <input type="radio"/>  |
| <b>I found the system unnecessarily complex.</b>                                                  | <input type="radio"/>     | <input type="radio"/> | <input type="radio"/> | <input type="radio"/> | <input type="radio"/>  |
| <b>I thought the system was easy to use.</b>                                                      | <input type="radio"/>     | <input type="radio"/> | <input type="radio"/> | <input type="radio"/> | <input type="radio"/>  |
| <b>I think that I would need the support of a technical person to be able to use this system.</b> | <input type="radio"/>     | <input type="radio"/> | <input type="radio"/> | <input type="radio"/> | <input type="radio"/>  |
| <b>I found the various functions in this system were well integrated.</b>                         | <input type="radio"/>     | <input type="radio"/> | <input type="radio"/> | <input type="radio"/> | <input type="radio"/>  |

2. \*

*Mark only one oval per row.*

|                                                                                      | 1<br>Strongly<br>Disagree | 2                     | 3                     | 4                     | 5<br>Strongly<br>Agree |
|--------------------------------------------------------------------------------------|---------------------------|-----------------------|-----------------------|-----------------------|------------------------|
| <b>I thought there was too much inconsistency in this system.</b>                    | <input type="radio"/>     | <input type="radio"/> | <input type="radio"/> | <input type="radio"/> | <input type="radio"/>  |
| <b>I would imagine that most people would learn to use this system very quickly.</b> | <input type="radio"/>     | <input type="radio"/> | <input type="radio"/> | <input type="radio"/> | <input type="radio"/>  |
| <b>I found the system very cumbersome to use.</b>                                    | <input type="radio"/>     | <input type="radio"/> | <input type="radio"/> | <input type="radio"/> | <input type="radio"/>  |
| <b>I felt very confident using the system.</b>                                       | <input type="radio"/>     | <input type="radio"/> | <input type="radio"/> | <input type="radio"/> | <input type="radio"/>  |
| <b>I needed to learn a lot of things before I could get going with this system.</b>  | <input type="radio"/>     | <input type="radio"/> | <input type="radio"/> | <input type="radio"/> | <input type="radio"/>  |

3. Terminology:

\*

**Data case** refers to an instance of the data set; synonymous with data item or data point.

**Attribute** refers to properties of the data cases in the data set; synonymous with feature, dimension, or variable.

**Relationship in the data** refers to attributes among the data, such as correlations, clusters, or distributions.

Please use N/A if you think an item is not applicable

Mark only one oval per row.

|                                                                                                                               | Strongly<br>Disagree  | Disagree              | Somewhat<br>Disagree  | Neither<br>Agree<br>nor<br>Disagree | Somewhat<br>Agree     | Agree                 | Strongly<br>Agree     | N/A                   |
|-------------------------------------------------------------------------------------------------------------------------------|-----------------------|-----------------------|-----------------------|-------------------------------------|-----------------------|-----------------------|-----------------------|-----------------------|
| The visualization exposes individual data cases and their attributes                                                          | <input type="radio"/> | <input type="radio"/> | <input type="radio"/> | <input type="radio"/>               | <input type="radio"/> | <input type="radio"/> | <input type="radio"/> | <input type="radio"/> |
| The visualization facilitates perceiving relationships in the data like patterns & distributions of the variables             | <input type="radio"/> | <input type="radio"/> | <input type="radio"/> | <input type="radio"/>               | <input type="radio"/> | <input type="radio"/> | <input type="radio"/> | <input type="radio"/> |
| The visualization promotes exploring relationships between individual data cases as well as different groupings of data cases | <input type="radio"/> | <input type="radio"/> | <input type="radio"/> | <input type="radio"/>               | <input type="radio"/> | <input type="radio"/> | <input type="radio"/> | <input type="radio"/> |

4. \*

Mark only one oval per row.

|                                                                                                          | Strongly<br>Disagree  | Disagree              | Somewhat<br>Disagree  | Neither<br>Agree<br>nor<br>Disagree | Somewhat<br>Agree     | Agree                 | Strongly<br>Agree     | N/A                   |
|----------------------------------------------------------------------------------------------------------|-----------------------|-----------------------|-----------------------|-------------------------------------|-----------------------|-----------------------|-----------------------|-----------------------|
| <b>The visualization helps generate data-driven questions</b>                                            | <input type="radio"/> | <input type="radio"/> | <input type="radio"/> | <input type="radio"/>               | <input type="radio"/> | <input type="radio"/> | <input type="radio"/> | <input type="radio"/> |
| <b>The visualization helps identify unusual or unexpected, yet valid, data characteristics or values</b> | <input type="radio"/> | <input type="radio"/> | <input type="radio"/> | <input type="radio"/>               | <input type="radio"/> | <input type="radio"/> | <input type="radio"/> | <input type="radio"/> |

5. \*

Mark only one oval per row.

|                                                                                                          | Strongly<br>Disagree  | Disagree              | Somewhat<br>Disagree  | Neither<br>Agree<br>nor<br>Disagree | Somewhat<br>Agree     | Agree                 | Strongly<br>Agree     | N/A                   |
|----------------------------------------------------------------------------------------------------------|-----------------------|-----------------------|-----------------------|-------------------------------------|-----------------------|-----------------------|-----------------------|-----------------------|
| The visualization provides useful interactive capabilities to help investigate the data in multiple ways | <input type="radio"/> | <input type="radio"/> | <input type="radio"/> | <input type="radio"/>               | <input type="radio"/> | <input type="radio"/> | <input type="radio"/> | <input type="radio"/> |
| The visualization shows multiple perspectives about the data                                             | <input type="radio"/> | <input type="radio"/> | <input type="radio"/> | <input type="radio"/>               | <input type="radio"/> | <input type="radio"/> | <input type="radio"/> | <input type="radio"/> |

6. \*

Mark only one oval per row.

|                                                                                                                    | Strongly<br>Disagree  | Disagree              | Somewhat<br>Disagree  | Neither<br>Agree<br>nor<br>Disagree | Somewhat<br>Agree     | Agree                 | Strongly<br>Agree     | N/A                   |
|--------------------------------------------------------------------------------------------------------------------|-----------------------|-----------------------|-----------------------|-------------------------------------|-----------------------|-----------------------|-----------------------|-----------------------|
| The visualization uses an effective representation of the data that shows related and partially related data cases | <input type="radio"/> | <input type="radio"/> | <input type="radio"/> | <input type="radio"/>               | <input type="radio"/> | <input type="radio"/> | <input type="radio"/> | <input type="radio"/> |
| The visualization provides a meaningful spatial organization of the data                                           | <input type="radio"/> | <input type="radio"/> | <input type="radio"/> | <input type="radio"/>               | <input type="radio"/> | <input type="radio"/> | <input type="radio"/> | <input type="radio"/> |
| The visualization shows key characteristics of the data at a glance                                                | <input type="radio"/> | <input type="radio"/> | <input type="radio"/> | <input type="radio"/>               | <input type="radio"/> | <input type="radio"/> | <input type="radio"/> | <input type="radio"/> |

7. \*

Mark only one oval per row.

|                                                                                                            | Strongly<br>Disagree  | Disagree              | Somewhat<br>Disagree  | Neither<br>Agree<br>nor<br>Disagree | Somewhat<br>Agree     | Agree                 | Strongly<br>Agree     | N/A                   |
|------------------------------------------------------------------------------------------------------------|-----------------------|-----------------------|-----------------------|-------------------------------------|-----------------------|-----------------------|-----------------------|-----------------------|
| The interface supports using different attributes of the data to reorganize the visualization's appearance | <input type="radio"/> | <input type="radio"/> | <input type="radio"/> | <input type="radio"/>               | <input type="radio"/> | <input type="radio"/> | <input type="radio"/> | <input type="radio"/> |
| The visualization supports smooth transitions between different levels of detail in viewing the data       | <input type="radio"/> | <input type="radio"/> | <input type="radio"/> | <input type="radio"/>               | <input type="radio"/> | <input type="radio"/> | <input type="radio"/> | <input type="radio"/> |

8. \*

Mark only one oval per row.

|                                                                                                                            | Strongly<br>Disagree  | Disagree              | Somewhat<br>Disagree  | Neither<br>Agree<br>nor<br>Disagree | Somewhat<br>Agree     | Agree                 | Strongly<br>Agree     | N/A                   |
|----------------------------------------------------------------------------------------------------------------------------|-----------------------|-----------------------|-----------------------|-------------------------------------|-----------------------|-----------------------|-----------------------|-----------------------|
| The visualization avoids complex commands and textual queries by providing direct interaction with the data representation | <input type="radio"/> | <input type="radio"/> | <input type="radio"/> | <input type="radio"/>               | <input type="radio"/> | <input type="radio"/> | <input type="radio"/> | <input type="radio"/> |
| The visualization provides a comprehensive and accessible overview of the data                                             | <input type="radio"/> | <input type="radio"/> | <input type="radio"/> | <input type="radio"/>               | <input type="radio"/> | <input type="radio"/> | <input type="radio"/> | <input type="radio"/> |
| The visualization presents the data by providing a meaningful visual schema                                                | <input type="radio"/> | <input type="radio"/> | <input type="radio"/> | <input type="radio"/>               | <input type="radio"/> | <input type="radio"/> | <input type="radio"/> | <input type="radio"/> |



9. \*

Mark only one oval per row.

|                                                                                                         | Strongly<br>Disagree  | Disagree              | Somewhat<br>Disagree  | Neither<br>Agree<br>nor<br>Disagree | Somewhat<br>Agree     | Agree                 | Strongly<br>Agree     | N/A                   |
|---------------------------------------------------------------------------------------------------------|-----------------------|-----------------------|-----------------------|-------------------------------------|-----------------------|-----------------------|-----------------------|-----------------------|
| The visualization facilitates generalizations and extrapolations of patterns and conclusions            | <input type="radio"/> | <input type="radio"/> | <input type="radio"/> | <input type="radio"/>               | <input type="radio"/> | <input type="radio"/> | <input type="radio"/> | <input type="radio"/> |
| The visualization helps understand how variables relate in order to accomplish different analytic tasks | <input type="radio"/> | <input type="radio"/> | <input type="radio"/> | <input type="radio"/>               | <input type="radio"/> | <input type="radio"/> | <input type="radio"/> | <input type="radio"/> |
| The visualization uses meaningful and accurate visual encodings to represent the data                   | <input type="radio"/> | <input type="radio"/> | <input type="radio"/> | <input type="radio"/>               | <input type="radio"/> | <input type="radio"/> | <input type="radio"/> | <input type="radio"/> |

10. \*

Mark only one oval per row.

|                                                                                                                                | Strongly<br>Disagree  | Disagree              | Somewhat<br>Disagree  | Neither<br>Agree<br>nor<br>Disagree | Somewhat<br>Agree     | Agree                 | Strongly<br>Agree     | N/A                   |
|--------------------------------------------------------------------------------------------------------------------------------|-----------------------|-----------------------|-----------------------|-------------------------------------|-----------------------|-----------------------|-----------------------|-----------------------|
| The visualization avoids using misleading representations                                                                      | <input type="radio"/> | <input type="radio"/> | <input type="radio"/> | <input type="radio"/>               | <input type="radio"/> | <input type="radio"/> | <input type="radio"/> | <input type="radio"/> |
| The visualization promotes understanding data domain characteristics beyond the individual data cases and attributes           | <input type="radio"/> | <input type="radio"/> | <input type="radio"/> | <input type="radio"/>               | <input type="radio"/> | <input type="radio"/> | <input type="radio"/> | <input type="radio"/> |
| If there were data issues like unexpected, duplicate, missing, or invalid data, the visualization would highlight those issues | <input type="radio"/> | <input type="radio"/> | <input type="radio"/> | <input type="radio"/>               | <input type="radio"/> | <input type="radio"/> | <input type="radio"/> | <input type="radio"/> |

This content is neither created nor endorsed by Google.

Google Forms
